# Supplementary material for: SeeGera: Self-supervised Semi-implicit Graph Variational Auto-encoders with Masking
Source: arXiv:2301.12458 source file (2023-02-07)
Supplement: Supplementary file 1 [file appendix.tex]

\appendix
\section{Appendix}
\subsection{Dataset description}
We conducted extensive experiments on four public attributed networks.
Specifically,
\emph{Cora}~\cite{kipf2016semi}, \emph{Cora-ml}~\cite{bojchevski2017deep} and \emph{Citeseer}~\cite{kipf2016semi}
are citation networks,
whose nodes are publications and edges are citation links.
Attributes for each node are keywords it contains.
Each dimension in the attribute vector indicates the presence of a keyword in the publication.
For simplicity,
we omit edge directions and take these networks as undirected ones.
\emph{Facebook}~\cite{meng2019co} is a network dataset where nodes represent users and edges capture the friendship relation.
Attributes are constructed from user profiles.
Note that all the datasets have binary edges and attributes.
Moreover,
nodes in Cora, Cora-ml and Citeseer
are associated with labels that describe research topics of publications.
These three datasets are used in the node classification task.
Table~\ref{table:statistics} summarizes statistics of datasets used in our experiments.

\begin{table}[!htbp]
\caption{Statistics of datasets used in experiments}
\label{table:statistics}
\centering
\resizebox{0.9\linewidth}{!}
{
\begin{tabular}{c|ccccc} \hline
Datasets &  \#Nodes & \#Edges & \#Attributes & \#Labels  \\ \hline
Cora  & $2,708$ & $5,278$ & $1,433$ & $7$    \\ \hline
Cora-ml  & $2,995$ & $8,158$ & $2,879$ & $7$ \\ \hline
Citeseer & $3,327$ & $4,676$ & $3,703$ & $6$    \\ \hline 
Facebook & $4,039$ & $88,234$ & $1,406$ & $-$  \\ \hline
\end{tabular}
}
\end{table}

\subsection{Implementation details}
We implemented \algo\ by Tensorflow.
The model is initialized by Glorot initialization and trained by Adam.
We run the model for 3500 epochs with the learning rate 0.0005 on all the datasets.
%We set the layer size of both GCN and MLP in the inference model to be $[128, 64]$.
We set 
%In the inference model of \algo,
both GCN and MLP in the inference model to have two layers with size equal to $[128, 64]$.
We choose Bernoulli noise for both $\tilde{\epsilon} \sim \tilde{q}({\epsilon})$ and $\hat{\epsilon} \sim \hat{q}({\epsilon})$.
We fine tune the noise dimension by grid search over $\{4, 8, 16, 32, 64\}$.
In the tasks of link prediction and node classification,
we set the dimension of injected noise to be 4 for the stochastic layer in both GCN and MLP.
In the attribute inference task, 
we set it to be 64.
As suggested by~\cite{sonderby2016ladder},
we use 
warm-up during the first 300 epochs 
to gradually impose the prior regularization terms $\mathrm{D_{KL}} (q_{1}(\rmzv | \psi_1) || p(\rmzv))$
and $\mathrm{D_{KL}} (q_{2}(\rmza | \psi_2) || p(\rmza))$.
Further,
since $\rma$ and $\rmx$ are sparse in our experiments,
we re-weight terms with $\rma_{ij} = 1$ and $\rmx_{ir} = 1$ as in~\cite{kipf2016variational}.
For both priors $p(\rmzv)$ and $p(\rmza)$,
we assume that they follow standard multivariate normal distributions.
%$\mathcal{N}(0,I)$, where $I$ is the identity matrix.
%While large values of $J$ and $K$ in Eq.~\ref{eq:reweight} drive $\underl_K^{J}$ close to $\log (\rma, \rmx)$,
%it will cost a large amount of computational resources.
For fair comparison,
we set the embedding dimension for all the methods to be 64
and 
%use the same early stopping strategy for graph neural network based methods.
run all the experiments on a single NVIDIA 1080Ti GPU.
For simplicity,
we set $J = K = 1$ in Eq.~\ref{eq:reweight} for both \algo\ and SIG-VAE.
One may further refer to~\cite{rainforth2018tighter} for better value selection.
For all the baseline methods, we use the original codes released by their authors
and fine tune the model parameters.
%We also adopt the same early stopping strategy as \algo.
For random-walk-based methods,
we set the window size to 10,
the walk length to 80, 
the number of walks per node to 10, and the number of negative samples to 5.

\subsection{Complexity analysis}
The model includes an inference model and a generative model.
The major computation cost in the inference model comes from the two-layer GCN and the two-layer MLP.
Let $|\tilde{\rma}^{+}|$ be the number of non-zero entries in the graph Laplacian matrix,
$l$ be the number of attributes,
$d_1$ be the hidden layer dimension and $d$ be the output layer dimension.
Further,
we denote $\tilde{d}$ and $\hat{d}$ as the dimensions of injected noise to the GCN and MLP, respectively.
For GCN,
the time complexity is 
$O(|\tilde{\rma}^{+}|(l+\tilde{d}+d_1) + n (l+\tilde{d}) d_1 + n d_1 d)$.
For MLP, 
the time complexity is
$O(l(n+\hat{d})d_1 + ld_1d)$.
In our experiments,
the attribute matrix $\rmx$ is also sparse,
so the time complexities reduce to 
$O(|\tilde{\rma}^{+}|(l+\tilde{d}+d_1) + |\rmx^+| d_1 + n\tilde{d}d_1 + n d_1 d)$
and
$O(|\rmx^+| d_1 + l\hat{d} d + l d_1 d)$,
where $|\rmx^+|$ is the number of non-zero entries in the attribute matrix $\rmx$.
In the inference process,
we run GCN and MLP $J+K$ times in total.
For the generative model,
the time complexity of generating the adjacency matrix $\rma$ is $O(n^2d)$
while that of reconstructing the attribute matrix $\rmx$ is $O(lnd)$.
Specifically,
we run the generative model $J$ times in total.
Empirically,
we observe that \algo\ costs around 2.84s, 6.42s, 9.19s, 5.88s per 100 epochs on Cora, Cora-ml, Citeseer and Facebook, respectively.

\subsection{Lower bound for ELBO}
To derive the ELBO in Eq.~\ref{eq:elbo} under the hierarchical variational framework,
we define $h_{\phi}(\rmzv, \rmza) = \int_{\psi_1} \int_{\psi_2} q(\rmzv, \rmza |\psi_1, \psi_2)q_{\phi}(\psi_1, \psi_2) \rmd \psi_1 \rmd \psi_2$ 
as the marginal distribution over $\rmzv$ and $\rmza$.
Then we use Jensen's inequality and have:
%$z \sim q(z | \psi)$, $\psi \sim q_{\phi}(\psi)$, $z \sim h_{\phi}(z) = \int_{\psi} q(z|\psi)q_{\phi}(\psi) d \psi$
\begin{equation}
\begin{split}
\log p(\rma, \rmx) & = \log \int_{\rmzv} \int_{\rmza} p (\rma,\rmx,\rmzv,\rmza)\rmd\rmzv \rmd \rmza \\
& = \log \int_{\rmzv} \int_{\rmza} p (\rma,\rmx, \rmzv, \rmza) \frac{h_{\phi}(\rmzv, \rmza)}{h_{\phi}(\rmzv, \rmza)} \rmd\rmzv \rmd \rmza \\
& \geq \mathbb{E}_{h_{\phi}(\rmzv, \rmza)} \left [ \log \frac{p (\rma,\rmx,\rmzv,\rmza)}{h_{\phi}(\rmzv, \rmza)} \right ]\\ 
\end{split}
\end{equation}
However, 
since $h_{\phi}$ is generally intractable,
the Monte Carlo estimation for the ELBO could be prohibited. 
%\begin{equation}
%\text{KL}(\mathbb{E}_{\psi}q(\rmz | \psi) || p(\rmz)) \leq \mathbb{E}_{\psi} \text{KL}(q(\rmz | \psi ) || p(\rmz)).
%\end{equation}.
We thus derive a lower bound $\underl$ in Eq.~\ref{eq:underll} for the ELBO:
\begin{equation}
\nonumber
\small
\begin{split}
\mathcal{L}  & = \mathbb{E}_{h_{\phi}(\rmzv, \rmza)} \left [ \log \frac{p (\rma,\rmx,\rmzv,\rmza)}{h_{\phi}(\rmzv, \rmza)} \right ]\\ 
& = \mathbb{E}_{h_{\phi_1}(\rmzv)} \mathbb{E}_{h_{\phi_2}(\rmza)} \left [ \log \frac{p (\rmzv | \rma,\rmx) p(\rmza| \rmx^T)p(\rma,\rmx)}{h_{\phi_1}(\rmzv) h_{\phi_2}(\rmza)} \right ]\\ 
& = - \mathbb{E}_{h_{\phi_1}(\rmzv)} \left [ \log \frac{h_{\phi_1}(\rmzv)}{p (\rmzv | \rma,\rmx)} \right ] - \mathbb{E}_{h_{\phi_2}(\rmza)} \left [ \log \frac{h_{\phi_2}(\rmza)}{p(\rmza| \rmx ^ T)} \right ] + \log p(\rma,\rmx) \\
& = -\mathrm{D_{KL}} (h_{\phi_1}(\rmzv) || p (\rmzv | \rma, \rmx)) -\mathrm{D_{KL}} (h_{\phi_2}(\rmza) || p (\rmza | \rmx ^ T))+ \log p(\rma,\rmx)\\ 
& \geq -\mathbb{E}_{\psi_1 \sim q_{\phi_1}(\psi_1)} \mathrm{D_{KL}} (q_{1}(\rmzv | \psi_1) || p (\rmzv | \rma, \rmx)) \\
& \quad - \mathbb{E}_{\psi_2 \sim q_{\phi_2}(\psi_2)} \mathrm{D_{KL}} (q_{2}(\rmza | \psi_2) || p (\rmza | \rmx^T)) + \log p(\rma,\rmx) \\
& = \mathbb{E}_{\psi_1 \sim q_{\phi_1}(\psi)}\mathbb{E}_{\rmzv \sim q_{1}(\rmzv | \psi_1)}\mathbb{E}_{\psi_2 \sim q_{\phi_2}(\psi)}\mathbb{E}_{\rmza \sim q_{2}(\rmza | \psi_2)}\\
& \quad \left [ \log \frac{p (\rma,\rmx,\rmzv,\rmza)}{q_{1}(\rmzv | \psi_1)q_{2}(\rmza | \psi_2)}\right ] \\
& = \underl \\
\end{split}
\end{equation}
where $\mathrm{D_{KL}}$ is the KL divergence
and
we employ 
$\mathrm{D_{KL}}(\mathbb{E}_{\psi}q(\rmz | \psi) || p(\rmz)) \leq \mathbb{E}_{\psi} \mathrm{D_{KL}}(q(\rmz | \psi ) || p(\rmz))$
according to~\cite{pmlr-v80-yin18b}.
In $\underl$,
$q_1$ and $q_2$ are required to have analytic density function,
while
$q_{\phi_1}$ and $q_{\phi_2}$ could be implicit but have to be convenient to be sampled from.
%It is thus easier to optimize $\underl$.
Directly optimizing $\underl$ by Monte Carlo Estimation is much easier.
Moreover, $\underl$ can be expanded to derive Eq.~\ref{eq:underl_expand}:
%We have the variational distribution as:
%\begin{equation}
%h_{\phi}(\rmzv, \rmza | \rma,\rmx) = \prod_{i \in \mathcal{V}} h_{\phi_1}(\rmzv_i | \rma, \rmx) \prod_{a \in \mathcal{A}} h_{\phi_2}(\rmza_a | \rmx^T)
%\end{equation}
%
%\begin{equation}
%p (\rma,\rmx,\rmzv,\rmza) = p(\rmzv) p(\rmza) \prod_{i,j \in \mathcal{V}} p(\rma_{ij}| \rmzv_i, \rmzv_j) \prod_{i \in \mathcal{V}, j \in \mathcal{A}}p(\rmx_{ij} | \rmzv_i, \rmza_j)
%\end{equation}
\begin{equation}
\nonumber
\begin{split}
\underl & = \mathbb{E}_{\psi_1 \sim q_{\phi_1}(\psi)}\mathbb{E}_{\rmzv \sim q_{1}(\rmzv | \psi_1)}\mathbb{E}_{\psi_2 \sim q_{\phi_2}(\psi)}\mathbb{E}_{\rmza \sim q_{2}(\rmza | \psi_2)} \\
&\quad \left [ \log \frac{p(\rmzv)p(\rmza) p(\rma | \rmzv)p(\rmx | \rmza, \rmza)}{q_{1}(\rmzv | \psi_1)q_{2}(\rmza | \psi_2)}\right ] \\
%\log p(\rma, \rmx) & \geq \mathbb{E}_{h_{\phi}(\rmzv, \rmza | \rma,\rmx)} \left [\sum_{i,j \in \mathcal{V}} \log p(\rma_{ij}| \rmzv_i, \rmzv_j) \right ]\\ 
%& + \mathbb{E}_{h_{\phi}(\rmzv, \rmza | \rma,\rmx)} \left [\sum_{i \in \mathcal{V}, j \in \mathcal{A}} \log p(\rmx_{ij}| \rmzv_i, \rmza_j) \right ]\\ 
%& - \mathrm{D_{KL}} (h_{\phi_1}(\rmzv | \rma, \rmx) || p(\rmzv))\\
%& - \mathrm{D_{KL}} (h_{\phi_2}(\rmza | \rmx^{T}) || p(\rmza))\\
& =  \mathbb{E}_{\psi \sim q_{\phi_1}(\psi)}\mathbb{E}_{\rmzv \sim q_{\theta_1}(\rmzv | \psi)} \left [\sum_{i,j \in \mathcal{V}} \log p(\rma_{ij}| \rmzv_i, \rmzv_j) \right ]\\ 
& \quad + \mathbb{E}_{\psi_1 \sim q_{\phi_1}(\psi)}\mathbb{E}_{\rmzv \sim q_{\theta_1}(\rmzv | \psi_1)}\mathbb{E}_{\psi_2 \sim q_{\phi_2}(\psi)}\mathbb{E}_{\rmza \sim q_{\theta_2}(\rmza | \psi_2)} \\
&\quad \quad \left [\sum_{i \in \mathcal{V}, r \in \mathcal{A}} \log p(\rmx_{ij}| \rmzv_i, \rmza_r) \right ]\\ 
&\quad  - \mathbb{E}_{\psi_1 \sim q_{\phi_1}(\psi)} \mathrm{D_{KL}} (q_{1}(\rmzv | \psi_1) || p(\rmzv))\\
& \quad - \mathbb{E}_{\psi_2 \sim q_{\phi_2}(\psi)} \mathrm{D_{KL}} (q_{2}(\rmza | \psi_2) || p(\rmza)).\\
\end{split}
\end{equation}

%\begin{equation}
%\small
%\begin{split}
%L & = \mathbb{E}_{((\rmzv)_1, (\rmza)_1, \psi_1^1, \psi_2^1), \ldots, ((\rmzv)_J, (\rmza)_J, \psi_1^J, \psi_2^J) \sim q(\rmzv, \rmza | \psi_1, \psi_2) q(\psi_1, \psi_2) } \mathbb{E}_{(\psi_1^{(1)}, \psi_2^{(1)}), \ldots, (\psi_1^{(K)}, \psi_2^{(K)}) \sim q_{\phi}(\psi_1, \psi_2)} \\
%& \log \frac{1}{J} \sum_{i=1}^J \frac{p(\rma, \rmx, (\rmzv)_i, (\rmza)_i)}{\frac{1}{K+1}\left[ q((\rmzv)_i, (\rmza)_i | \psi_1, \psi_2) + \sum_{k=1}^K q((\rmzv)_i, (\rmza)_i | \psi_1^{(k)}, \psi_2^{(k)}) \right]}\\
%\end{split}
%\end{equation}

\subsection{Algorithm}
We first rewrite Eq~\ref{eq:reweight} as 
\begin{equation}
\label{eq}
\begin{split}
\underl_K^{J} 
%& = \mathbb{E}_{\{(\rmzv)_j, (\rmza)_j, \psi_1^j, \psi_2^j\}_{j=1}^J \sim q(\rmzv, \rmza | \psi_1, \psi_2) q_{\phi}(\psi_1, \psi_2) } \mathbb{E}_{\{\tilde{\psi}_1^{k}, \tilde{\psi}_2^{k}\}_{k=1}^K \sim q_{\phi}(\psi_1, \psi_2)} \\
%& \log \frac{1}{J} \sum_{j=1}^J \frac{p(\rma, \rmx, (\rmzv)_j, (\rmza)_j)}{\frac{1}{K+1}\left[ q((\rmzv)_j, (\rmza)_j | \psi_1^j, \psi_2^j) + \sum_{k=1}^K q((\rmzv)_j, (\rmza)_j | \tilde{\psi}_1^{k}, \tilde{\psi}_2^{k}) \right]}\\
& = \mathbb{E}_{\{(\rmzv)_j, (\rmza)_j, \psi_1^j, \psi_2^j\}_{j=1}^J \sim q(\rmzv, \rmza | \psi_1, \psi_2) q_{\phi}(\psi_1, \psi_2) } \\
& \quad \mathbb{E}_{\{\tilde{\psi}_1^{k}, \tilde{\psi}_2^{k}\}_{k=1}^K \sim q_{\phi}(\psi_1, \psi_2)}  \log \frac{1}{J} \sum_{j=1}^J e ^ {\Upsilon_j - \Omega_j}.\\
\end{split}
\end{equation}
where $\Upsilon_j = \log p(\rma, \rmx, (\rmzv)_j, (\rmza)_j)$ and 
\begin{equation}
\nonumber
\small
\Omega_j = \log \frac{1}{K+1}\left[ q((\rmzv)_j, (\rmza)_j | \psi_1^j, \psi_2^j) + \sum_{k=1}^K q((\rmzv)_j, (\rmza)_j | \tilde{\psi}_1^{k}, \tilde{\psi}_2^{k}) \right]
 \end{equation}

%For $\log p(\rma, \rmx, (\rmzv)_j, (\rmza)_j)$, we omit the subscript for brevity and have
%\begin{equation}
%\begin{split}
%\log p(\rma, \rmx, \rmzv, \rmza) & = \log p(\rma | \rmzv) + \log p(\rmx | \rmzv, \rmza) + \log p(\rmzv) + \log p(\rmza) \\
%& = \sum_{i,j = 1}^n \log p(\rma_{ij} | \rmzv_i, \rmzv_j) + \sum_{i=1}^n \sum_{r=1}^l \log p(\rmx_{ir} | \rmzv_i, \rmza_r)\\
%& \quad - \frac{1}{2} \sum_{i=1}^n \sum_{k=1}^d ({\rmzv_{ij}})^2 - \frac{1}{2}  \sum_{i=1}^n \sum_{k=1}^d ({\rmza_{ik}})^2 + const \\
%\end{split}
%\end{equation}

%For $q((\rmzv)_j, (\rmza)_j | \psi_1^j, \psi_2^j)$, 
%we expand it as 
%$q((\rmzv)_j, (\rmza)_j | \psi_1^j, \psi_2^j) = q_1((\rmzv)_j | \psi_1^j)q_2((\rmza)_j | \psi_2^j)$, where $q_1$ and $q_2$ are multivariate normal distribution.
Then we summarize the Monte Carlo estimation for Eq.~\ref{eq} and the pseudocode of \algo\ in Alg.~\ref{alg:hoane}.
Here we denote $\psi_1 = [\muv, \Sigmav]$ and $\psi_2 = [\mua, \Sigmaa]$.
We also use neural networks $T_{\phi_1}(\rma, \rmx, \epsilon_1)$ and $T_{\phi_2}(\rmx^T, \epsilon_2)$ to represent $q_{\phi_1}$ and $q_{\phi_2}$, respectively.
\begin{algorithm}[H]
%\begin{small}
\begin{algorithmic}[1]
\Require $\rma$, $\rmx$, $q_1(\rmzv | \psi_1)$, $q_2(\rmza | \psi_2)$,
%explicit variational distributions $q_1(\rmzv | \psi_1)$ and $q_2(\rmza | \psi_2)$ with reparameterization functions $\rmzv = f(\psi_1)$ and $\rmza = g(\psi_2)$,
$T_{\phi_1}(\rma, \rmx, \epsilon_1)$, $T_{\phi_2}(\rmx^T, \epsilon_2)$, $\tilde{q}({\epsilon})$, $\hat{q}({\epsilon})$, learning rate $\rho$
\Ensure $\phi_1$ and $\phi_2$
\State Initialize $\phi_1$, $\phi_2$, set $\underl_K^J = 0$
\While{not converged}
\For{$k = 1$ \text{to} $K$}
\State Sample $\tilde{\psi}_1^k = T_{\phi_1}(\rma, \rmx, \tilde{\epsilon}_1^k)$, \text{where} $\tilde{\epsilon}_1^k \sim \tilde{q}({\epsilon})$
\State Sample $\tilde{\psi}_2^k = T_{\phi_2}(\rmx^T, \hat{\epsilon}_2^k)$, \text{where} $\hat{\epsilon}_2^k \sim \hat{q}({\epsilon})$
\EndFor
%\State Sample $\tilde{\psi}_1^k = T_{\phi_1}(\rma, \rmx, \tilde{\epsilon}_1^k)$, $\tilde{\epsilon}_1^k \sim \tilde{q}({\epsilon})$, $\tilde{\psi}_2^k = T_{\phi_2}(\rmx^T, \hat{\epsilon}_2^k)$, $\hat{\epsilon}_2^k \sim \hat{q}({\epsilon})$ for $k = 1, \cdots, K$
%\State Sample $\tilde{\psi}_2^k = T(\rmx^T, \hat{\epsilon}^k)$, $\hat{\epsilon}^k \sim \hat{q}(\hat{\epsilon})$ for $k = 1, \cdots, K$
\For{$j=1$ \text{to} $J$}
\State Sample $\psi_1^j = [(\muv)_j, (\Sigmav)_j] = T_{\phi_1}(\rma, \rmx, {{\epsilon}}_1^j)$, ${{\epsilon}}_1^j \sim \tilde{q}({\epsilon})$
\State Sample $\psi_2^j = [(\mua)_j, (\Sigmaa)_j] = T_{\phi_2}(\rmx^T, {{\epsilon}}_2^j)$, ${{\epsilon}}_2^j \sim \hat{q}({\epsilon})$
%\State Sample $\psi_2^j = T(\rmx^T, \tilde{\epsilon}^j)$, $\hat{\epsilon}^j \sim \hat{q}(\hat{\epsilon})$
%\State Sample $(\rmzv)_j = f(\psi_1^j)$ and $(\rmza)_j = g(\psi_2^j)$
%\LeftComment{Sample $\rmzv$ and $\rmza$ based on $\psi_1^j$ and $\psi_2^j$}
\State Sample $\epsilon_j^{\mathcal{V}} \sim \mathcal{N}(0, I)$, $\epsilon_j^{\mathcal{A}} \sim \mathcal{N}(0, I)$ 
\State Sample $(\rmzv)_j = (\muv)_j + (\Sigmav)_j \odot \epsilon_j^{\mathcal{V}}$ 
\State Sample $(\rmza)_j = (\mua)_j + (\Sigmaa)_j \odot \epsilon_j^{\mathcal{A}}$ 
%\State  Set $tmp_1 = -\log \frac{1}{K+1} \left[q((\rmzv)_j, (\rmza)_j | \psi_1^j, \psi_2^j) + \sum_{k=1}^K q((\rmzv)_j, (\rmza)_j | \tilde{\psi}_1^{k}, \tilde{\psi}_2^{k})\right] $
\State  Set $tmp_1 = - \Omega_j$
%\Comment{Note that $q((\rmzv)_j, (\rmza)_j | \psi_1^j, \psi_2^j) = q_1((\rmzv)_j | \psi_1^j)q_2((\rmza)_j | \psi_2^j)$ with $q_1 \sim \mathcal{N}((\muv)_j, (\Sigmav)_j)$ and $q_2 \sim \mathcal{N}((\mua)_j, (\Sigmaa)_j)$}
%\State  Set $tmp_2 = -\log \frac{1}{K+1}\left[\sum_{k=1}^K q_2((\rmza)_j | \tilde{\psi}_2^{k}) + q_2((\rmza)_j | \psi_2^j) \right] $
\State  Set $tmp_2 = \log p(\rma | \rmzv) + \log p(\rmx | \rmzv, \rmza) $ %\Comment{generate $\rma$ and $\rmx$ by Eq.~\ref{eq:decoder}}
\State  Set $tmp_3 = \log p(\rmzv) + \log p(\rmza)$ %\Comment{priors are standard normal distribution}
\State Update $\underl_K^J = \underl_K^J + e^{tmp_1 + tmp_2 + tmp_3 } $
\EndFor 
%\State Update $\underl_K^J$ by Eq.~\ref{eq:reweight}
\State Update $\underl_K^J = \log \underl_K^J - \log J$
\State Update $\phi_1 = \phi_1 + \rho \triangledown_{\phi_1} \underl_K^J $ %(\{ \tilde{\psi}_1^k, \tilde{\psi}_2^k\}_{k=1}^K, \{{\psi}_1^j, {\psi}_2^j, (\rmzv)_j, (\rmza)_j\}_{j=1}^J)$
\State Update $\phi_2 = \phi_2 + \rho \triangledown_{\phi_2} \underl_K^J $ %(\{ \tilde{\psi}_1^k, \tilde{\psi}_2^k\}_{k=1}^K, \{{\psi}_1^j, {\psi}_2^j, (\rmzv)_j, (\rmza)_j\}_{j=1}^J)$
\EndWhile
\State \Return $\phi_1$ and $\phi_2$
\end{algorithmic}
%\end{small}
\caption{\algo}
\label{alg:hoane}
\end{algorithm}
In Line 8,
$q((\rmzv)_j, (\rmza)_j | \psi_1^j, \psi_2^j) = q_1((\rmzv)_j | \psi_1^j)q_2((\rmza)_j | \psi_2^j)$ with $q_1 \sim \mathcal{N}((\muv)_j, (\Sigmav)_j)$ and $q_2 \sim \mathcal{N}((\mua)_j, (\Sigmaa)_j)$.
In Line 9,
%$\sum_{i,j = 1}^n \log p(\rma_{ij} | \rmzv_i, \rmzv_j) + \sum_{i=1}^n \sum_{r=1}^l \log p(\rmx_{ir} | \rmzv_i, \rmza_r)$.
$\rma$ and $\rmx$ are generated by Eq.~\ref{eq:decoder}.
In Line 10,
$p(\rmzv)$ and $p(\rmza)$ follow standard multivariate normal distribution.
